# Supplementary material for: Nonlinear Flexoelectricity in Non-centrosymmetric Crystals
Source: arXiv:1702.02740 ancillary file (2017-02-09)
Supplement: Supplementary file 1 [file Supplemental_Material.pdf]

# Supplementary Material

Kanghyun Chu, and Chan-Ho Yang

## 1 Detailed calculation process of the elastic and dielectric constants of the one-dimensional ionic chain system

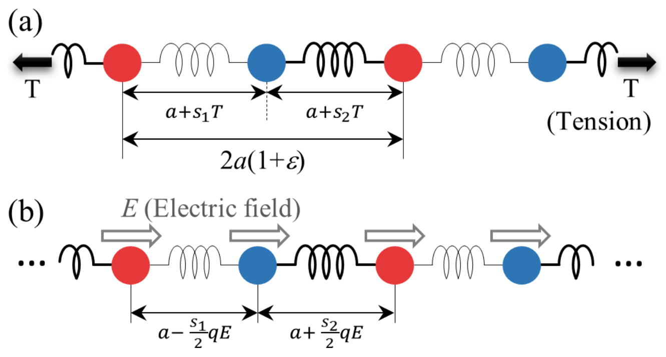


Figure S1: Response of the one-dimensional ionic chain system under the (a) uniform tension and the (b) uniform electric field.

Provided a tension $T$ is applied to the system as shown in the Figure S1(a), the lengths ($L_1$ and $L_2$) of the springs $k_1$ and $k_2$ are changed to

$$\begin{aligned} L_1 &= a + s_1 T \\ L_2 &= a + s_2 T. \end{aligned} \tag{1}$$

The strain $\varepsilon$ - the ratio of the length change to the original length - is given by

$$\varepsilon = \frac{1}{2a}(s_1 + s_2)T. \tag{2}$$

Therefore, the mechanical coefficient which is defined as the ratio of the strain to the tension is obtained as the following

$$\frac{\varepsilon}{T} = \frac{1}{2a}(s_1 + s_2). \tag{3}$$

As shown in the Figure S1(b), an external electric field $E$ applies a force to each individual ion, $\pm qE$. Considering the force balance at each ion, the tension force difference between the springs is also $\pm qE$, *i.e.*

$$T_{k_1} + qE = T_{k_2}, \tag{4}$$

where the $T_{k_1}$ and $T_{k_2}$ are the tensions of the springs $k_1$ and $k_2$, respectively. They can be written as

$$\begin{aligned} T_{k_1} &= T_o - \frac{1}{2}qE \\ T_{k_2} &= T_o + \frac{1}{2}qE. \end{aligned} \tag{5}$$

Then, the lengths of the springs can be expressed as

$$\begin{aligned} L_1 &= a + s_1(T_o - \frac{1}{2}qE) \\ L_2 &= a + s_2(T_o + \frac{1}{2}qE), \end{aligned} \tag{6}$$

where $s_1$ and the $s_2$ are the inverse of the spring constants. For simplicity, the pristine tension $T_o$ is assumed to be zero. It means that there is no external tension force acting on the system.

Considering a unit cell containing the positive ion on the left and the negative ion on the right so that the initial dipole moment $p^0_{\text{u.c.}}$ is $-qa$, the induced dipole moment per unit cell is

$$\begin{aligned} \Delta p_{\text{u.c.}} &= -qL_1 - p^0_{\text{u.c.}} \\ &= \frac{1}{2}q^2 s_1 E. \end{aligned} \tag{7}$$

We can rearrange the equation by adding and subtracting the factor $\frac{1}{4}q^2 s_2 E$, *i.e.*

$$\begin{aligned} \Delta p_{\text{u.c.}} &= \frac{1}{2}q^2 s_1 E + \frac{1}{4}q^2 s_2 E - \frac{1}{4}q^2 s_2 E \quad = \frac{q^2}{4}(s_1 + s_2)E + (-qa)\frac{qE}{4a}(s_2 - s_1) \\ &= \frac{q^2}{4}(s_1 + s_2)E + p^0_{\text{u.c.}}\varepsilon(E). \end{aligned} \tag{8}$$

Note that the strain $\varepsilon$ is the length change of the system$(-\frac{1}{2}s_1 qE + \frac{1}{2}s_2 qE)$ over the original length of unit cell$(2a)$, and it is non-zero when the system is non-centrosymmetric. (It is noteworthy that, this term is related to the converse piezoelectric effect.) The alternative unit cell where the negative ion is on the left and the positive ion is on the right gives $p^0_{\text{u.c.}} = qa$. Irrespective of the unit cell, the induced dipole is expressed in the same form, *i.e.*

$$\begin{aligned} \Delta p_{\text{u.c.}} &= qL_2 - p^0_{\text{u.c.}} \\ &= \frac{1}{2}q^2 s_2 E \\ &= \frac{q^2}{4}(s_1 + s_2)E + (qa)\frac{qE}{4a}(s_2 - s_1) \\ &= \frac{q^2}{4}(s_1 + s_2)E + p^0_{\text{u.c.}}\varepsilon(E). \end{aligned} \tag{9}$$

The first term $\frac{q^2}{4}(s_1+s_2)E$ represents the dielectric effect. The second term $p^0_{\text{u.c.}}\varepsilon(E)$ is the extrinsic piezoelectric term that says there is dipole moment change when a system whose initial dipole moment is non-zero undergoes the deformation. If the dipole free unit cell ($p^0_{\text{u.c.}} = 0$) is utilized, the calculation process becomes simple because the extrinsic piezoelectric term is eliminated.

$$\begin{aligned} \Delta p_{\text{u.c.}} &= -qL_1 + \frac{q}{2}(L_1 + L_2) \\ &= \frac{q^2}{4}(s_1 + s_2)E. \end{aligned} \tag{10}$$

Therefore, the induced dipole moment per unit cell normalized by the electric field is

$$\frac{\Delta p_{\text{u.c.}}}{E} = \frac{q^2}{4}(s_1 + s_2). \tag{11}$$

## 2 Homogeneous strain gradient and the corresponding displacement vector field in the continuum limit

Let $\vec{u}(\vec{r})$ be the displacement vector field that describes the position change of a body element initially at the position $\vec{r}$ due to a deformation. The strain tensor is defined as the symmetrized derivatives of the displacement vector field with respect to position in the infinitesimal strain limit, *i.e.*

$$\varepsilon_{ij} = \frac{1}{2}(\partial_i u_j + \partial_j u_i), \tag{12}$$

where $i, j$ are the spatial coordinate indices and $\partial_i$ is the partial derivative operator along the $i$-axis. Suppose a spatially uniform strain gradient and then the $\vec{u}(\vec{r})$ is expressed as a quadratic form of position. For two-dimensional cases, the displacement vector field is written as the following equation:

$$\begin{aligned} u_x(x,y)\big(\equiv u(x,y)\big) &= \frac{1}{2}s_{11}x^2 + \frac{1}{2}s_{12}y^2 + s_{13}xy \\ u_y(x,y)\big(\equiv v(x,y)\big) &= \frac{1}{2}s_{21}x^2 + \frac{1}{2}s_{22}y^2 + s_{23}xy. \end{aligned} \tag{13}$$

The coefficients $s_{ij}$ describes a deformation of the entire system subject to a uniform strain gradient, where the first subscript $i$ stands for the coordinates $x$ or $y$ and the second $j$ follows the Voigt notation in two-dimensional systems (*i.e.* $1 = xx, 2 = yy, 3 = xy$). The coefficients are uniquely specified by constraints associated with a given strain gradient. On the basis of this expression, we can get the position-dependent strain as below.

$$\begin{aligned} \varepsilon_{xx}(x,y) &= s_{11}x + s_{13}y \\ \varepsilon_{yy}(x,y) &= s_{22}y + s_{23}x \\ 2\varepsilon_{xy}(x,y) &= (s_{13}+s_{21})x + (s_{12}+s_{23})y \end{aligned} \tag{14}$$

Following the convention of the shear strain $\gamma_{xy} = 2\varepsilon_{xy}$, we can obtain the six components of the strain gradient tensor in the two-dimensional case, *i.e.*,

$$\begin{aligned} \partial_x\varepsilon_{xx} &= s_{11} \\ \partial_x\varepsilon_{yy} &= s_{23} \\ \partial_x\gamma_{xy} &= s_{13} + s_{21} \\ \partial_y\varepsilon_{xx} &= s_{13} \\ \partial_y\varepsilon_{yy} &= s_{22} \\ \partial_y\gamma_{xy} &= s_{12} + s_{23}. \end{aligned} \tag{15}$$

In particular, when we consider a deformation where only the transverse strain gradient of $\frac{\partial}{\partial y}\varepsilon_{xx}$ is non-zero, the coefficients $s_{ij}$ should satisfy

$$\begin{aligned} s_{13} &= \acute{\varepsilon} \\ s_{21} &= -\acute{\varepsilon} \\ s_{11} = s_{12} = s_{22} = s_{23} &= 0, \end{aligned} \tag{16}$$

where the $\acute{\varepsilon}$ is the magnitude of the strain gradient. In the two dimensional ionic chain network simulation, the positions of the outermost fixed sites were determined according to the Equations 13 and 16.

In addition, the tilt of the local body element, *i.e* a rotation of the element around the out-of-plane axis with fixing the shape, is described as the anti-symmetric differential form:

$$\begin{aligned} \theta_{xy} &= \frac{1}{2}(\partial_x u_y - \partial_y u_x) \\ &= \frac{1}{2}\big((-s_{13}+s_{21})x + (s_{23}-s_{12})y\big). \end{aligned} \tag{17}$$

In the case of a homogeneous transverse strain gradient, the components of the tilt gradient are given by

$$\begin{aligned} \partial_x\theta_{xy} &= -\acute{\varepsilon} \\ \partial_y\theta_{xy} &= 0. \end{aligned} \tag{18}$$

It implies unit cells of which the $x$-positions are positive are rotated clockwise when $\acute{\varepsilon} > 0$.

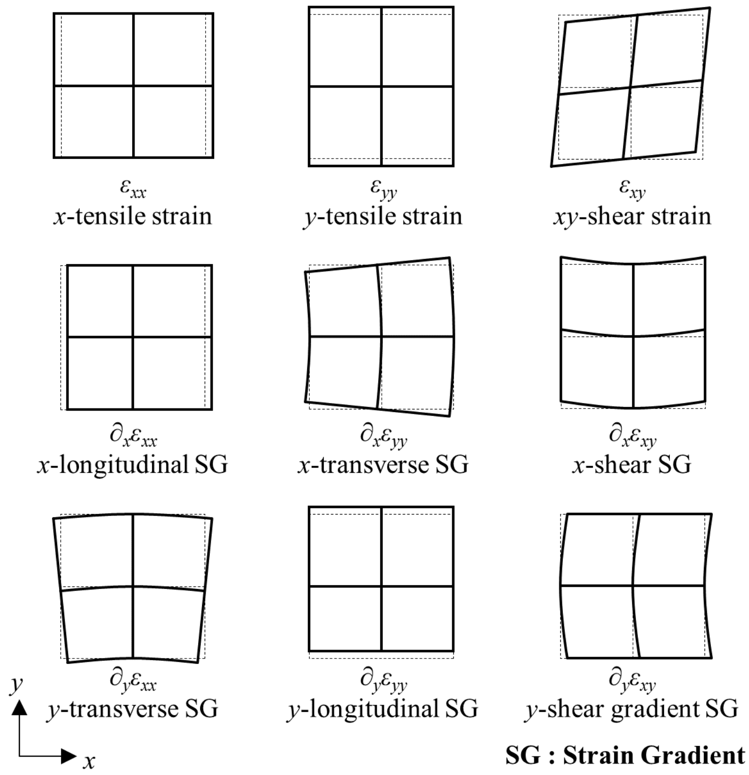


Figure S2: Schematic diagrams of each strain and strain gradient component in two-dimensional space.

# 3 Expressions of local strain, strain gradient, and pole moments using atomic scale ionic models

In the simulation study based on the ionic chain network model, the local strain states and local dipole moments of each relaxed configuration were analyzed. Here, the mathematical formulae in use for connecting the phenomenological quantities with the microscopic model are described. Consider a simple square cell of a side length $a$ and label its sites as the Figure S3. The deformation of the cell is described by the position of each ion at $(x_\alpha, y_\alpha)$ where $\alpha$ is the index to represent the ionic site. Let $\vec{u}_\alpha$ be the corresponding displacement vector that is given as

$$\vec{u}_\alpha = u_\alpha \hat{x} + v_\alpha \hat{y} = \big(x_\alpha - x_\alpha^0\big)\hat{x} + \big(y_\alpha - y_\alpha^0\big)\hat{y}, \tag{19}$$

where $\hat{x}$ and $\hat{y}$ are the unit vectors and $(x_\alpha^0, y_\alpha^0)$ is the initial position of the $\alpha$-th site before the deformation. Besides, the local strain of this cell is obtained by the finite difference form of Equation 12. For instance, $\varepsilon_{xx}$ is expressed as

$$\begin{aligned}\varepsilon_{xx} &= \frac{1}{2}\Big(\frac{u_3 - u_1}{a} + \frac{u_4 - u_2}{a}\Big) \\ &= \frac{1}{2a}(-u_1 - u_2 + u_3 + u_4).\end{aligned} \tag{20}$$

Since there are two equivalent pairs of sites that are 1&3 and 2&4, their mean value is taken. It can be also interpreted that the strain value is calculated based on the midpoints between 1&2 and 3&4. Similarly, the other strain components are expressed as

$$\begin{aligned}\varepsilon_{yy} &= \frac{1}{2a}(-v_1 + v_2 - v_3 + v_4) \\ \gamma_{xy} &= \frac{1}{2a}(-v_1 - v_2 + v_3 + v_4) + \frac{1}{2a}(-u_1 + u_2 - u_3 + u_4).\end{aligned} \tag{21}$$

This representation is extensionally applied to the pole-free cell. Each ionic site is labeled as the Figure S4. It is composed of four square sub-cells marked by A, B, C, and D. The strain state of the whole unit cell is taken as the average of the strain values of the sub-cells as like

$$\begin{aligned}\varepsilon_{xx} &= \frac{1}{4}\Big(\frac{1}{2a}(-u_1 - 2u_2 - u_3 + u_7 + 2u_8 + u_9)\Big) \\ \varepsilon_{yy} &= \frac{1}{4}\Big(\frac{1}{2a}(-v_1 + v_3 - 2v_4 + 2v_6 - v_7 + v_9)\Big) \\ \gamma_{xy} &= \frac{1}{4}\Big(\frac{1}{2a}(-v_1 - 2v_2 - v_3 + v_7 + 2v_8 + v_9) + \frac{1}{2a}(-u_1 + u_3 - 2u_4 + 2u_6 - u_7 + u_9)\Big).\end{aligned} \tag{22}$$

In the above equations, we note that only the outermost sites are involved and the inner site indexed by 5 is not shown in the formulae. It means the strain values represent the shape of the cell but do not carry any information of the internal ions. By considering the difference in the strain states of the sub-cells, one may calculate the strain gradient. For example, the derivative along the $x$-axis is taken as the mean difference between the pairs of A&C and B&D over the spacing $a$, *i.e.*

$$\frac{\Delta\varepsilon}{\Delta x} = \frac{1}{2}\Big(\frac{1}{a}(\varepsilon^C - \varepsilon^A) + \frac{1}{a}(\varepsilon^D - \varepsilon^B)\Big). \tag{23}$$

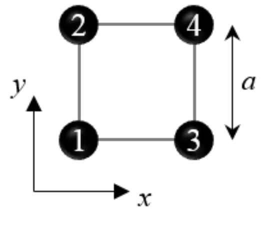


Figure S3: Square cell

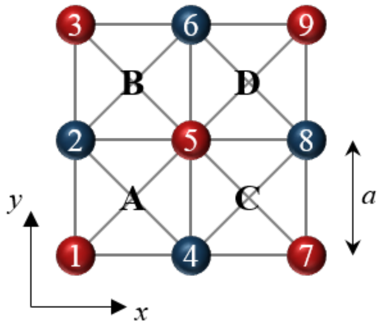


Figure S4: Indexing of ionic sites within the pole-free cell

For the $y$-derivatives, the pairings are swapped. All strain gradients are listed in the following equations.

$$\begin{aligned}
\frac{\Delta\varepsilon_{xx}}{\Delta x} &= \frac{1}{4a^2}(u_1 + 2u_2 + u_3 - 2u_4 - 4u_5 - 2u_6 + u_7 + 2u_8 + u_9) \\
\frac{\Delta\varepsilon_{yy}}{\Delta x} &= \frac{1}{4a^2}(v_1 - v_3 - v_7 + v_9) \\
\frac{\Delta\gamma_{xy}}{\Delta x} &= \frac{1}{4a^2}(u_1 - u_3 - u_7 + u_9 + v_1 + 2v_2 + v_3 - 2v_4 - 4v_5 - 2v_6 + v_7 + 2v_8 + v_9) \\
\frac{\Delta\varepsilon_{xx}}{\Delta y} &= \frac{1}{4a^2}(u_1 - u_3 - u_7 + u_9) \\
\frac{\Delta\varepsilon_{yy}}{\Delta y} &= \frac{1}{4a^2}(v_1 - 2v_2 + v_3 + 2v_4 - 4v_5 + 2v_6 + v_7 - 2v_8 + v_9) \\
\frac{\Delta\gamma_{xy}}{\Delta y} &= \frac{1}{4a^2}(u_1 - 2u_2 + u_3 + 2u_4 - 4u_5 + 2u_6 + u_7 - 2u_8 + u_9 + v_1 - v_3 - v_7 + v_9).
\end{aligned} \tag{24}$$

Note that only the transverse strain gradients of $\frac{\Delta\varepsilon_{yy}}{\Delta x}$ and $\frac{\Delta\varepsilon_{xx}}{\Delta y}$ are independent of the inner site information. In the same sense, the transverse strain gradients can be interpreted as the shape of the cell similarly to the strains. However, the other longitudinal ($\frac{\Delta\varepsilon_{xx}}{\Delta x}$, $\frac{\Delta\varepsilon_{yy}}{\Delta y}$) and shear ($\frac{\Delta\gamma_{xy}}{\Delta x}$, $\frac{\Delta\gamma_{xy}}{\Delta y}$) strain gradients are improper to describe the shape, but rather indicate the off-centering of the central ion. It gives rise to an ambiguity. Consider all the positive and negative ions shift along the rightward and leftward directions respectively. In that case, the signs of nominal longitudinal and shear strain gradients flip when an alternative pole-free cell whose center ion is negative is taken. Therefore, the longitudinal and shear strain gradients should be defined in the larger scale in the context of the strain difference between the adjacent pole-free cells.

The dipole moment of the system is given by the charge weighted sum of ionic positions. In that sense, each component of local dipole moment is written as

$$\begin{aligned}
p_x &= \sum_{\alpha=1}^{9} q_\alpha x_\alpha = \frac{q}{4}x_1 - \frac{q}{2}x_2 + \frac{q}{4}x_3 - \frac{q}{2}x_4 + qx_5 - \frac{q}{2}x_6 + \frac{q}{4}x_7 - \frac{q}{2}x_8 + \frac{q}{4}x_9 \\
p_y &= \sum_{\alpha=1}^{9} q_\alpha y_\alpha = \frac{q}{4}y_1 - \frac{q}{2}y_2 + \frac{q}{4}y_3 - \frac{q}{2}y_4 + qy_5 - \frac{q}{2}y_6 + \frac{q}{4}y_7 - \frac{q}{2}y_8 + \frac{q}{4}y_9.
\end{aligned} \tag{25}$$

If the pole-free cell is taken, the initial dipole moment of unperturbed system is zero and thus the induced dipole moment equals to the dipole moment itself. The following equation regarding the $x$-component expresses the argument in a mathematical form:

$$\Delta p_x = \sum_{\alpha=1}^{9} q_\alpha x_\alpha - \sum_{\alpha=1}^{9} q_\alpha x_\alpha^0 = \sum_{\alpha=1}^{9} q_\alpha x_\alpha - 0 = p_x. \tag{26}$$

Moreover, it is the same as the charge weighted sum of the displacement vectors.

$$p_x = \sum_{\alpha=1}^{9} q_\alpha x_\alpha - \sum_{\alpha=1}^{9} q_\alpha x_\alpha^0 = \sum_{\alpha=1}^{9} q_\alpha (x_\alpha - x_\alpha^0) = \sum_{\alpha=1}^{9} q_\alpha u_\alpha. \tag{27}$$

In the following, the elimination of the extrinsic piezoelectric and flexoelectric effects by choosing the pole-free cell will be explained. Assume that there is no internal strain and the displacement vector of each ion is

given as

$$u(x,y) = \frac{1}{2}s_{11}x^2 + \frac{1}{2}s_{12}y^2 + s_{13}xy + t_{11}x + t_{12}y$$
$$v(x,y) = \frac{1}{2}s_{21}x^2 + \frac{1}{2}s_{22}y^2 + s_{23}xy + t_{21}x + t_{22}y. \tag{28}$$

It is a more generalized form of the Equation 13 that also counts in a non-zero homogeneous strain governed by the $t_{ij}$ related terms, *i.e.*

$$\begin{aligned}\varepsilon_{xx}(x,y) &= s_{11}x + s_{13}y + t_{11}\\ \varepsilon_{yy}(x,y) &= s_{22}y + s_{23}x + t_{22}\\ \gamma_{xy}(x,y) &= (s_{13}+s_{21})x + (s_{12}+s_{23})y + t_{12} + t_{21}.\end{aligned} \tag{29}$$

The $x$-dipole moment at a position where the local unit cell is described by the unperturbed ionic positions is

$$\begin{aligned}p_x &= \sum_{\alpha=0}^{9} q_\alpha u(x^0_\alpha, y^0_\alpha)\\ &= \sum_{\alpha=0}^{9} q_\alpha \Big(\frac{1}{2}s_{11}(x^0_\alpha)^2 + \frac{1}{2}s_{12}(y^0_\alpha)^2 + s_{13}x^0_\alpha y^0_\alpha + t_{11}x^0_\alpha + t_{12}y^0_\alpha\Big).\end{aligned} \tag{30}$$

This equation is rearranged as the following:

$$\begin{aligned}p_x &= \frac{1}{2}s_{11}\sum_{\alpha=0}^{9} q_\alpha(x^0_\alpha)^2 + \frac{1}{2}s_{12}\sum_{\alpha=0}^{9} q_\alpha(y^0_\alpha)^2 + s_{13}\sum_{\alpha=0}^{9} q_\alpha x^0_\alpha y^0_\alpha + t_{11}\sum_{\alpha=0}^{9} q_\alpha x^0_\alpha + t_{12}\sum_{\alpha=0}^{9} q_\alpha y^0_\alpha\\ &= \frac{1}{2}Q^0_{xx}s_{11} + \frac{1}{2}Q^0_{yy}s_{12} + Q^0_{xy}s_{13} + p^0_x t_{11} + p^0_y t_{12},\end{aligned} \tag{31}$$

where the $Q^0_{ij}$ and $p^0_i$ are the non-traceless quadrupole moment and dipole moment of the unperturbed system that are all zeros in the pole-free cell. One may confirm it by plugging in the initial positions of ionic sites that are

$$\begin{aligned}x^0_1 = x^0_2 =& x^0_3 = x^0_5 - a\\ x^0_4 =& x^0_5 = x^0_6\\ x^0_7 = x^0_8 =& x^0_9 = x^0_5 + a\\ y^0_1 = y^0_4 =& y^0_7 = y^0_5 - a\\ y^0_2 =& y^0_5 = y^0_8\\ y^0_3 = y^0_6 =& y^0_9 = y^0_5 + a,\end{aligned} \tag{32}$$

and their charges of

$$\begin{aligned}q_1 = q_3 = q_7 = q_9 &= \frac{1}{4}q_5\\ q_2 = q_4 = q_6 = q_8 &= -\frac{1}{2}q_5.\end{aligned} \tag{33}$$

Therefore, no extrinsic effects enter into the calculation process when the pole-free cell is used. For the $y$-dipole moment, the same argument is made.

# 4 Calculation process for the piezoelectric coefficients

In this section, the process of obtaining the piezoelectric coefficients for the system of $k_{1x} = k_{2x} = 1$, $k_{1y} = 0.5264$, $k_{2y} = 10$, $k_p = k_n = 0.5$ is introduced. Various homogeneous strains are applied and the response of the dipole moment to each strain is analyzed. From the analyzed data, the induced dipole moment is expressed as a polynomial function of strain components. The coefficients of the function correspond to piezoelectric coefficients. Here, the tilt angle ($\theta_{xy}$) of the cell that is defined as the Equation 17 should be also regarded as an order parameter along with the strains because it induces a volume change of the cell as illustrated in the Figure S5, thereby contributing to the piezoelectric effect as much as a quadratic order of the angle. The tilted configuration of black solid circles and the original configuration of gray open circles have an identical nominal strain state, according to the Equations 20 and 21. The areas of the squares, however, are not equal to each other. There exists a quadratic contribution of $\theta_{xy}$ on the volume. The piezoelectric coefficients are quantities normalized by the volume and thus the volume change can influence the piezoelectric coefficients. Therefore, it is required to deal with it along with the strains $\varepsilon_{xx}, \varepsilon_{yy}, \gamma_{xy}$ when we handle the piezoelectric effect with second-order accuracy. At that time, the doubled value of $\theta_{xy}$ is used and denoted as $2\theta_{xy}$. The Taylor expansion of the local dipole moment induced by the small strains and tilt angle is generally written as the following form.

$$\begin{aligned}
p_x(\varepsilon_{xx},&\varepsilon_{yy},\gamma_{xy},2\theta_{xy})\\
&\simeq e_{x1}\varepsilon_{xx} + e_{x2}\varepsilon_{yy} + e_{x3}\gamma_{xy} + e_{x4}2\theta_{xy} + e_{x5}\varepsilon_{xx}^2 + e_{x6}\varepsilon_{yy}^2 + e_{x7}\gamma_{xy}^2 + e_{x8}(2\theta_{xy})^2\\
&\quad + e_{x9}\varepsilon_{xx}\varepsilon_{yy} + e_{x10}\varepsilon_{xx}\gamma_{xy} + e_{x11}\varepsilon_{yy}\gamma_{xy} + e_{x12}\varepsilon_{xx}2\theta_{xy} + e_{x13}\varepsilon_{yy}2\theta_{xy} + e_{x14}\gamma_{xy}2\theta_{xy} + O(\varepsilon^3, \theta_{xy}^3)\\
p_y(\varepsilon_{xx},&\varepsilon_{yy},\gamma_{xy},2\theta_{xy})\\
&\simeq e_{y1}\varepsilon_{xx} + e_{y2}\varepsilon_{yy} + e_{y3}\gamma_{xy} + e_{y4}2\theta_{xy} + e_{y5}\varepsilon_{xx}^2 + e_{y6}\varepsilon_{yy}^2 + e_{y7}\gamma_{xy}^2 + e_{y8}(2\theta_{xy})^2\\
&\quad + e_{y9}\varepsilon_{xx}\varepsilon_{yy} + e_{y10}\varepsilon_{xx}\gamma_{xy} + e_{y11}\varepsilon_{yy}\gamma_{xy} + e_{y12}\varepsilon_{xx}2\theta_{xy} + e_{y13}\varepsilon_{yy}2\theta_{xy} + e_{y14}\gamma_{xy}2\theta_{xy} + O(\varepsilon^3, \theta_{xy}^3)
\end{aligned} \tag{34}$$

Each of the extended piezoelectric coefficients $e_{ij}$ describes a response of the dipole moment to a variation of its conjugate pair of order parameters. The extended coefficients not only include the conventional piezoelectric coefficients but also contain extra ones arising from the quadratic expansion terms. Considering the symmetry of the system, some coefficients are taken to be zeros. The two-dimensional space group *cm* contains the mirror and glide symmetry operations as shown in the Figure S6. Considering the mirror symmetry, the coefficients of $e_{x1}$, $e_{x2}$, $e_{x5}$, $e_{x6}$, $e_{x7}$, $e_{x9}$, $e_{y3}$, $e_{y10}$, and $e_{y11}$ are zeros. In addition, the tilt angle does not contribute to the dipole moment in the linear order, because the tilt operation induces the $-x(+y)$ component by projecting the initial $y(x)$ dipole moment which is zero. Therefore, the $e_{x4}$ and $e_{y4}$ are also zeros. For the construction of sampling data to connect the order parameters to the dipole moment, the local dipole moment induced in the pole-free cell is numerically investigated for ten different types of a variation in order parameters and their quadratic combinations. Each strain component including the tilt angle is scanned individually from the value of -0.1 to +0.1 at an interval of 0.02 except for the zero strain case. From the Figure S7 to S10, the local dipole moment components and the corresponding local strains are displayed. Moreover, all the possible quadratic combinations of the strain parameters are varied simultaneously to get hints on the coefficients of the cross terms. From the Figure S11 to S16, the local dipole moment components and the strain states are displayed for each combination.

Collecting all the local dipole moment components with respect to the local strain states, each of the coefficients in Equation 34 is obtained by multi-variable fitting based on the least square method. Each relaxed configuration has nine cells at the central region. Each of the cells can be in a different state in terms of the local $\varepsilon_{xx}, \varepsilon_{yy}, \gamma_{xy}, 2\theta_{xy}$, which results in two $x$ and $y$ components of the local dipole moment according to the systems mechanoelectric property characterized by the $e_{ij}$ coefficients. Total 100 configurations (10 strain

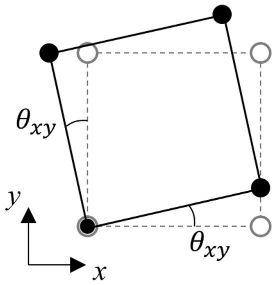


Figure S5: The tilt angle $\theta_{xy}$ and volume expansion of the cell. The gray dashed line square is the original configuration and the black bold line square is the tilted state of a non-zero $\theta_{xy}$.

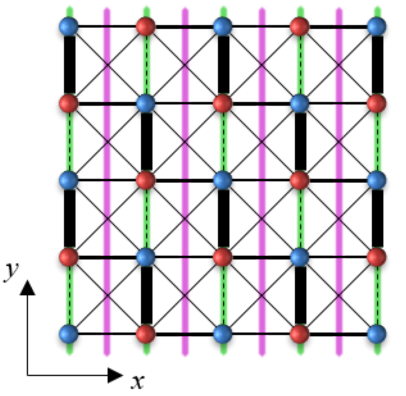


Figure S6: *cm* symmetry of the system. The green lines represent mirror lines and the magenta lines indicate glide lines

values $\times$ $(4+_4C_2)$ strain types and their combinations) were relaxed, thereby leading to 900 sampling data sets. Let $c_p$ be the 14-by-1 vector containing the extended piezoelectric coefficients related to the $p_x$ or $p_y$ as its components, $p$ be the 900-by-1 vector containing all the local $x$- or $y$-axis dipole moment data, and $S$ be the 900-by-14 matrix whose column vectors are local $\varepsilon_{xx}$, $\varepsilon_{yy}$, $\gamma_{xy}$, $2\theta_{xy}$, $\varepsilon_{xx}^2$, $\varepsilon_{yy}^2$, $\gamma_{xy}^2$, $(2\theta_{xy})^2$, $\varepsilon_{xx}\varepsilon_{yy}$, $\varepsilon_{xx}\gamma_{xy}$, $\varepsilon_{yy}\gamma_{xy}$, $\varepsilon_{xx}2\theta_{xy}$, $\varepsilon_{yy}2\theta_{xy}$, and $\gamma_{xy}2\theta_{xy}$. The $c_p$ can be determined from the $S$ and the $p$ by the least square method, *i.e.*

$$c_p = (S^T S)^{-1} S^T p. \tag{35}$$

Owing to the zero coefficients protected by the symmetry, we can efficiently reduce the dimensions of the $c_p$, $p$, and $S$, significantly relieving the computational complexity. The obtained coefficients are summarized in the Table S1. The bold zeros are the coefficients protected by the symmetry.

It is noteworthy that the value of the $e_{y2}$ agrees with the result of the linear chain model. The induced piezoelectric dipole moment per positive and negative ion pair is $qa\frac{s_2-s_1}{s_1+s_2}\varepsilon$ where the $s_{1,2}$ are the inverses of the spring constants $k_{1,2}$. Plugging in the values of $k_{1y}$ and the $k_{2y}$ into the $k_1$ and the $k_2$ respectively, the induced dipole moment value is $-0.9qa\varepsilon_{yy}$. Since the pole-free cell contains two pairs of positive and negative ions, the piezoelectric coefficient representing the inducement of $y$-dipole moment with respect to the tensile strain along the $y$ axis in the pole-free unit cell is doubled *i.e.* $-1.8qa$. Furthermore, the diagonal springs hardly affect the piezoelectric coefficient as shown in the Figure S17.

Table S1: Piezoelectric coefficients of the system of spring constants $k_{1x} = k_{2x} = 1$, $k_{1y} = 0.5264$, $k_{2y} = 10$ , $k_p = k_n = 0.5$. The unit of the coefficients is $qa$.

| $e_{x1}$ | $e_{x2}$ | $e_{x3}$ | $e_{x4}$ | $e_{x5}$ | $e_{x6}$ | $e_{x7}$ | $e_{x8}$ | $e_{x9}$ | $e_{x10}$ | $e_{x11}$ | $e_{x12}$ | $e_{x13}$ | $e_{x14}$ |
|---|---|---|---|---|---|---|---|---|---|---|---|---|---|
| **0** | **0** | -0.003 | **0** | **0** | **0** | **0** | -0.001 | **0** | -0.002 | 0.922 | 0.000 | 0.893 | 0.001 |
| $e_{y1}$ | $e_{y2}$ | $e_{y3}$ | $e_{y4}$ | $e_{y5}$ | $e_{y6}$ | $e_{y7}$ | $e_{y8}$ | $e_{y9}$ | $e_{y10}$ | $e_{y11}$ | $e_{y12}$ | $e_{y13}$ | $e_{y14}$ |
| 0.000 | -1.800 | **0** | **0** | -0.001 | 0.005 | -0.223 | -0.225 | 0.340 | **0** | **0** | 0.001 | -0.004 | 0.448 |

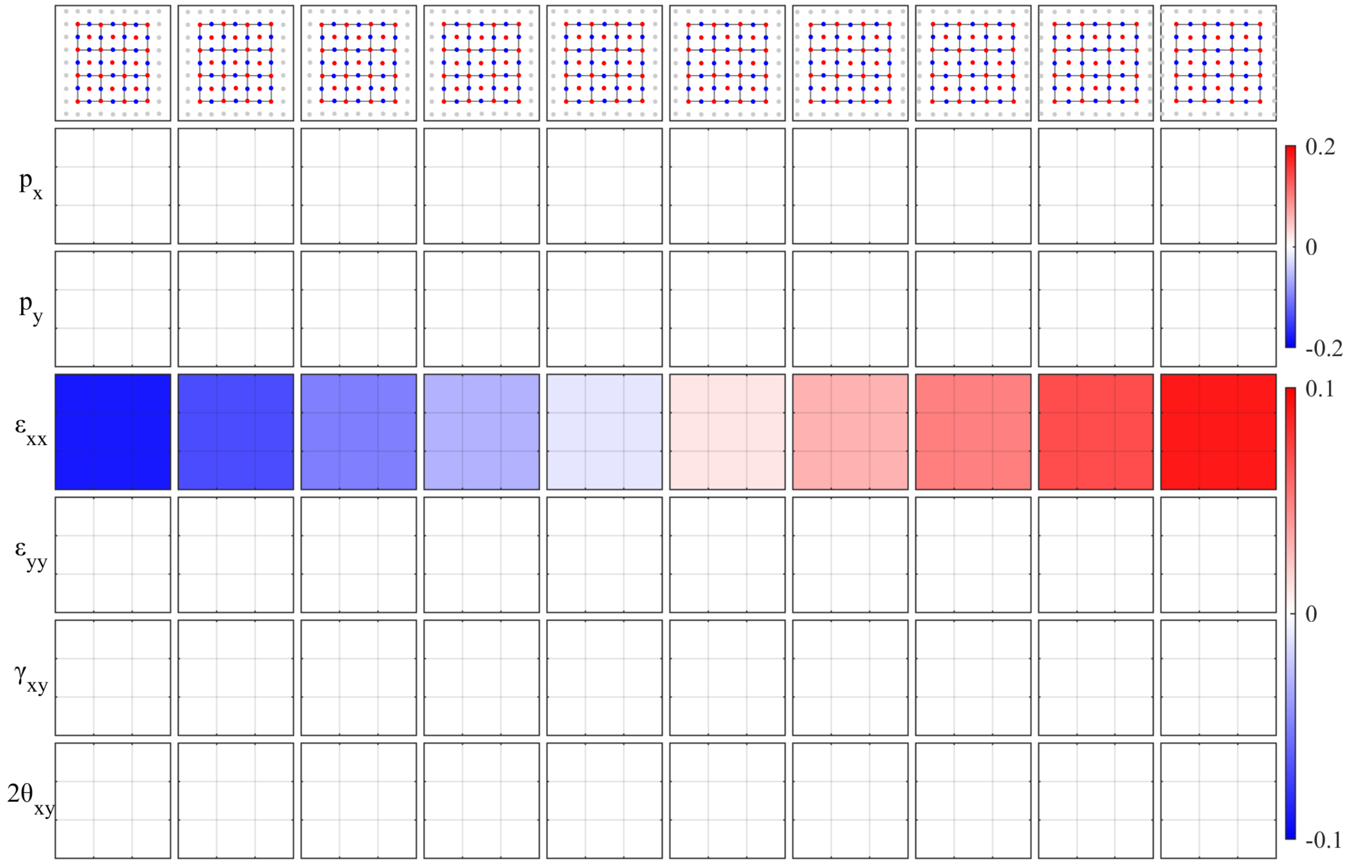


Figure S7: Changing $\varepsilon_{xx}$

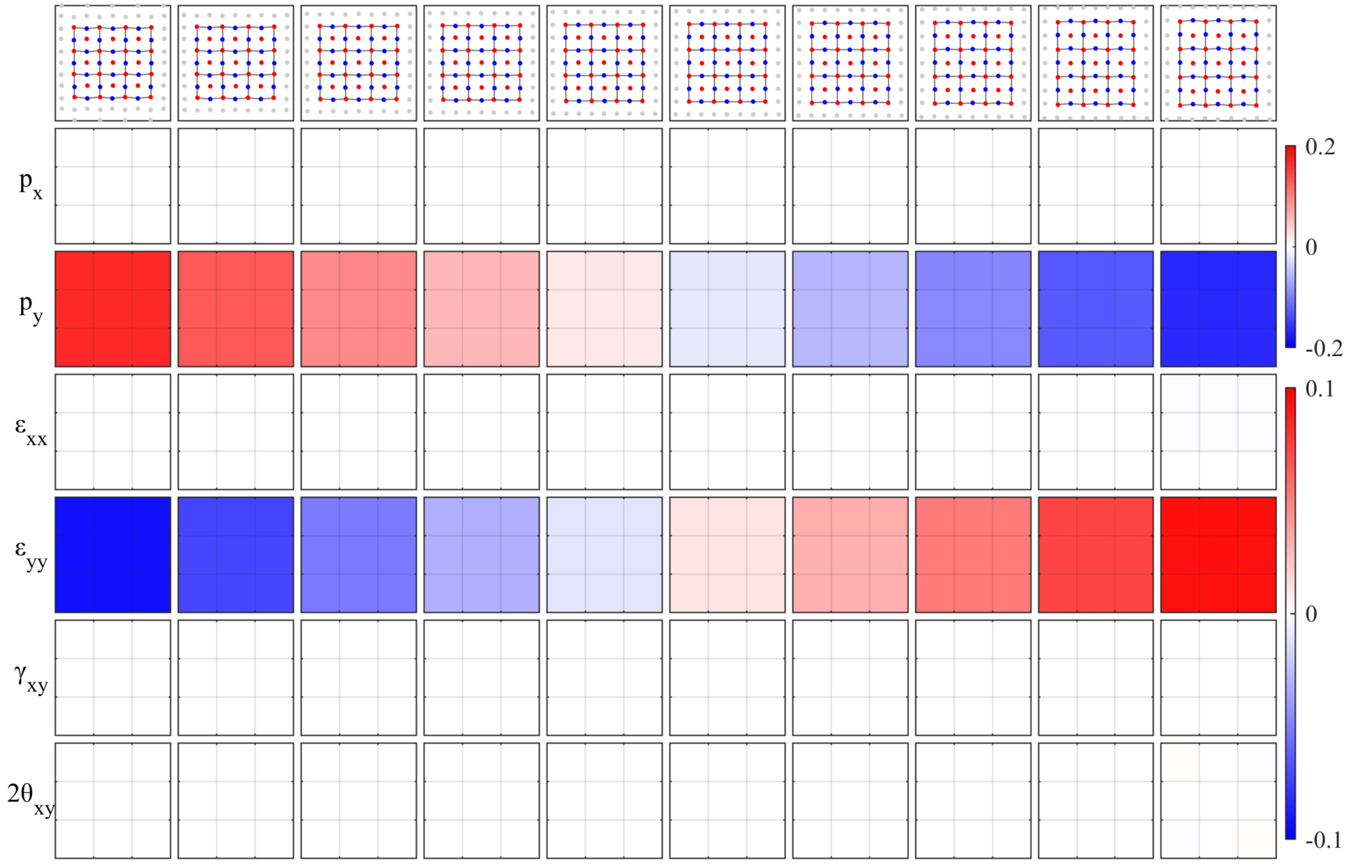


Figure S8: Changing $\varepsilon_{yy}$

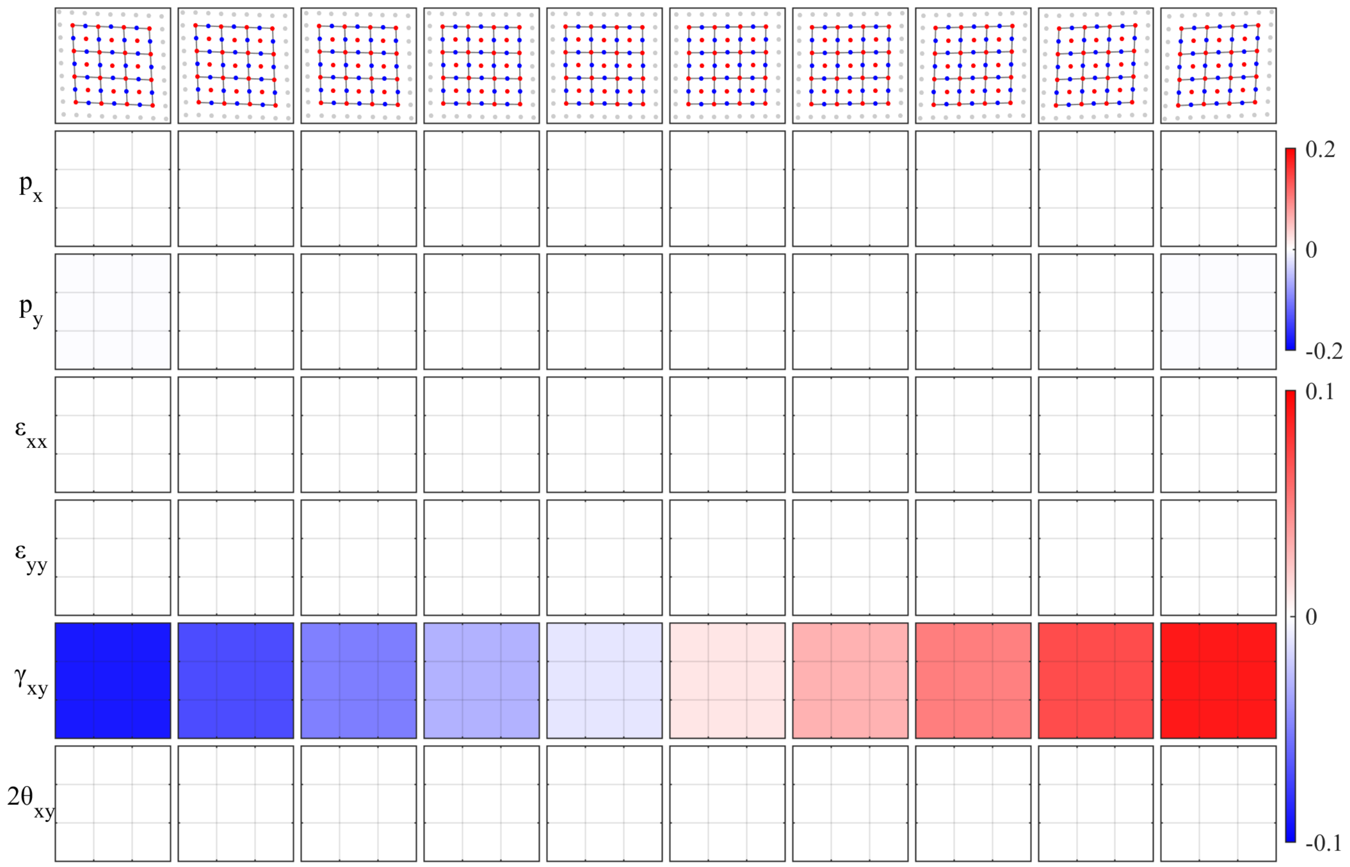


Figure S9: Changing $\gamma_{xy}$

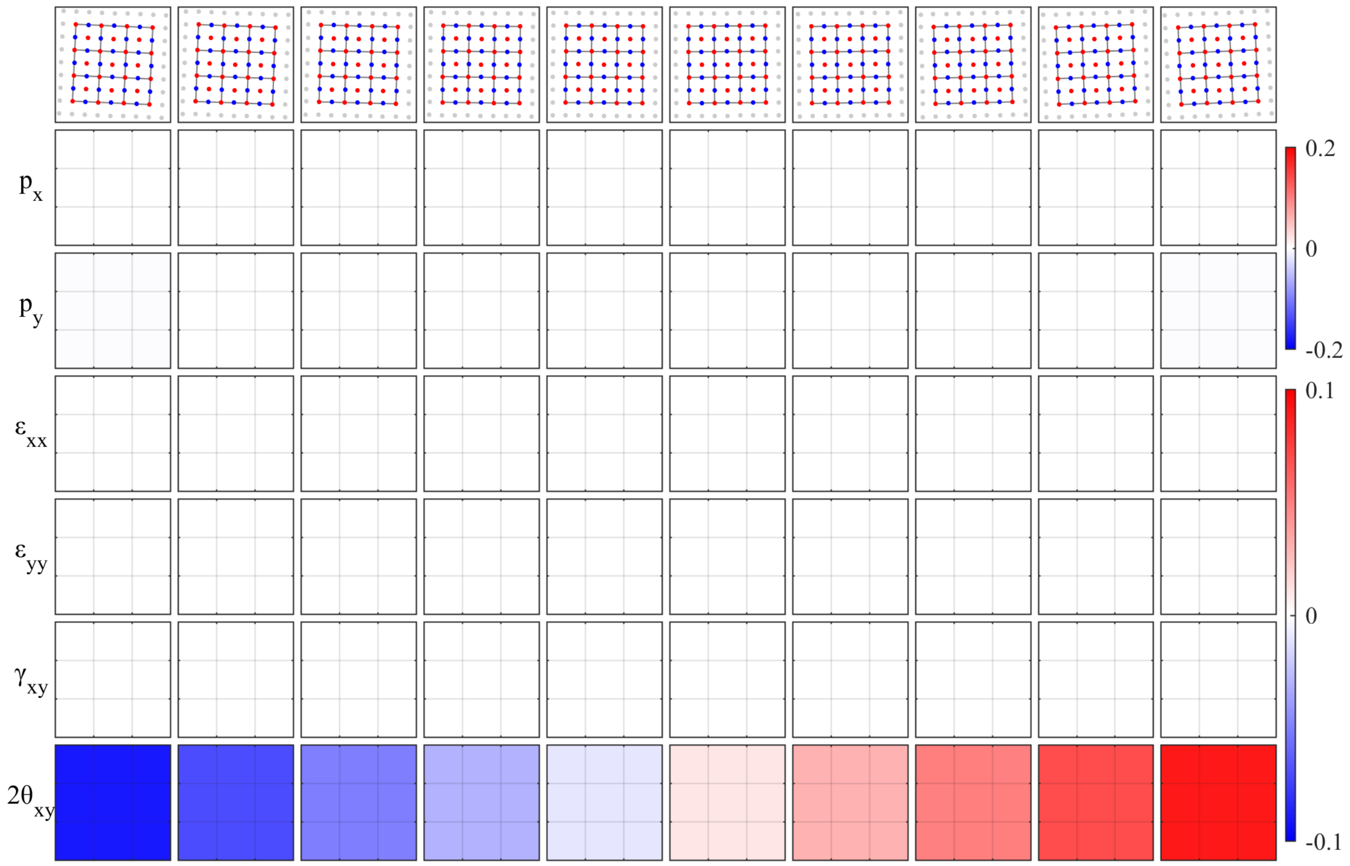


Figure S10: Changing $2\theta_{xy}$

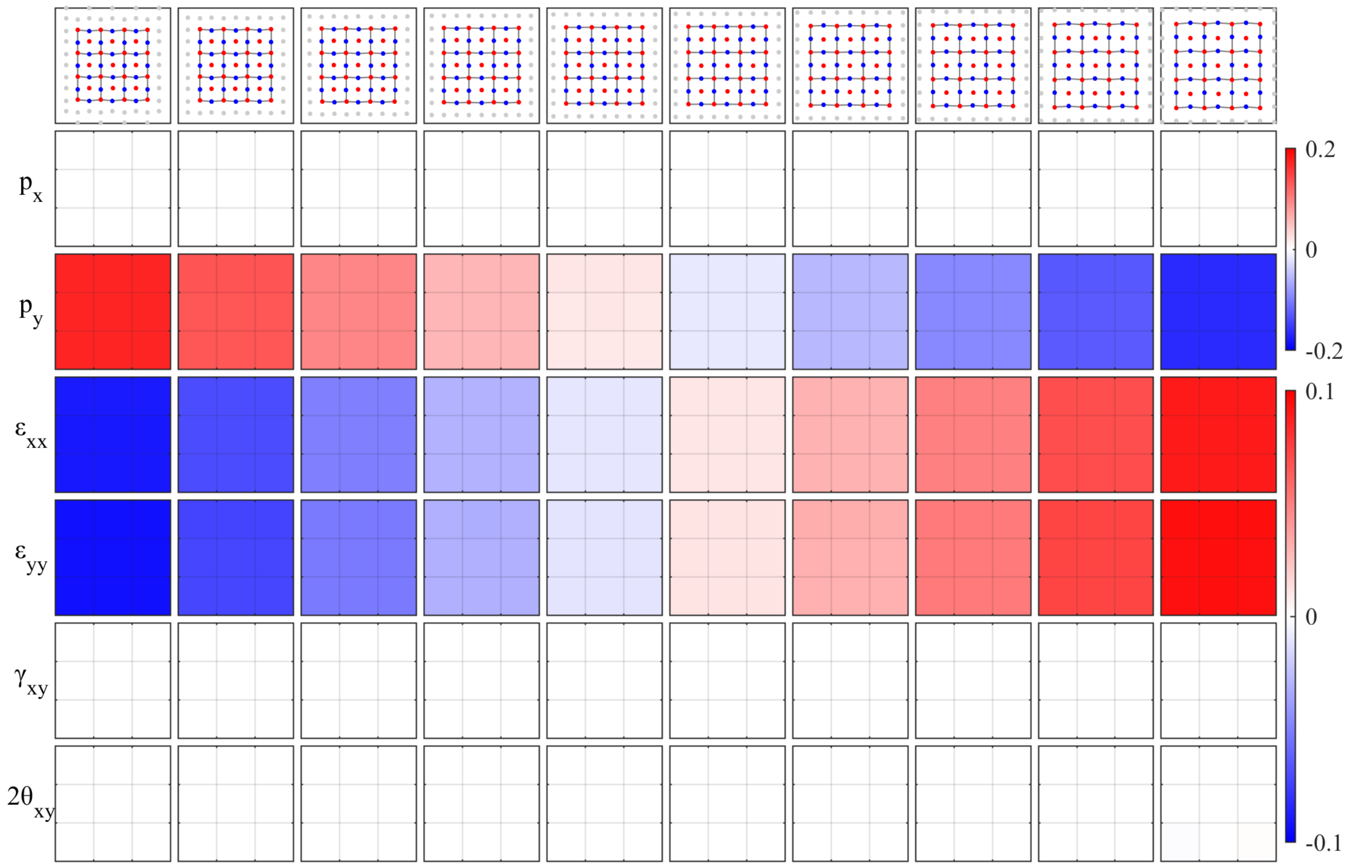


Figure S11: Changing $\varepsilon_{xx}$ and $\varepsilon_{yy}$ equally

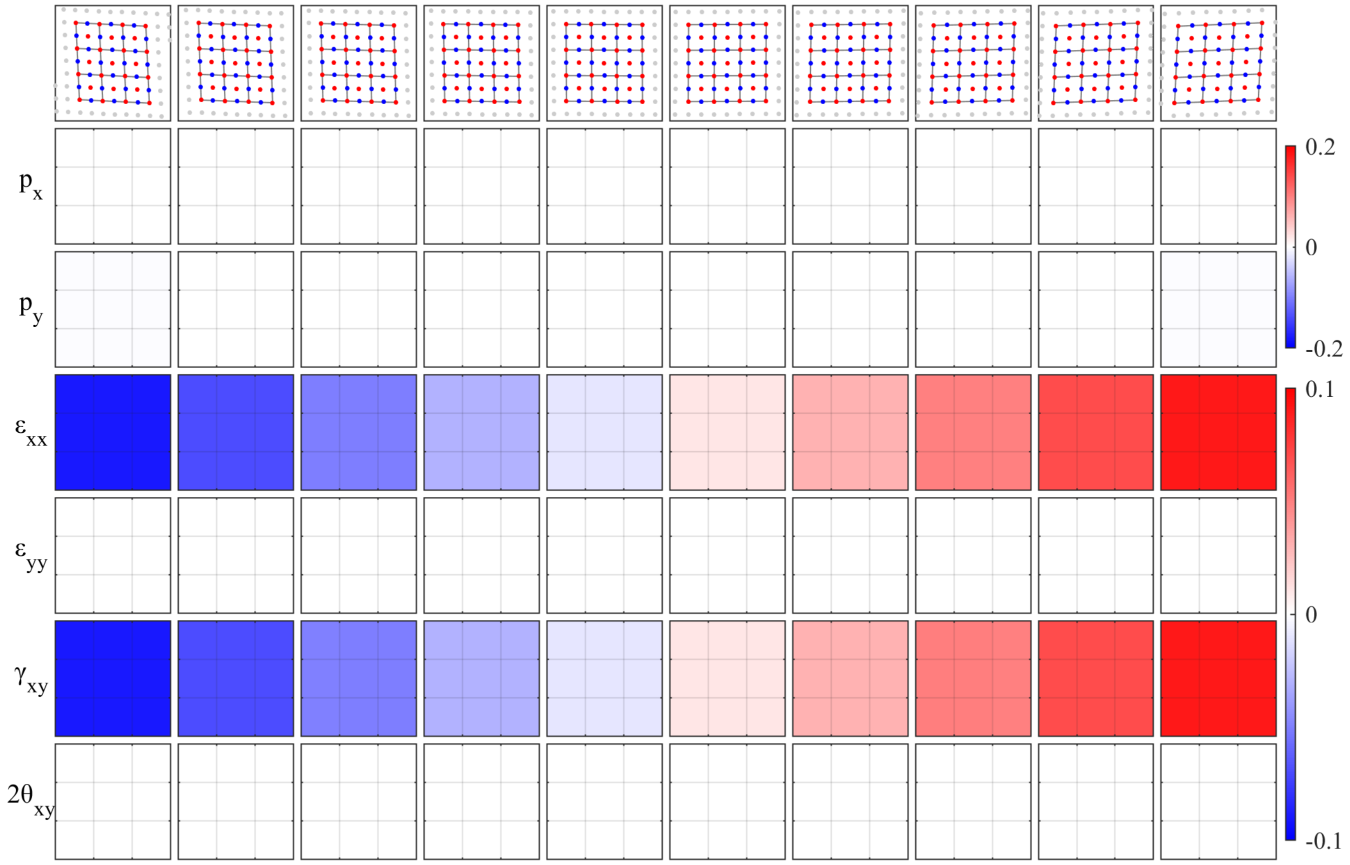


Figure S12: Changing $\varepsilon_{xx}$ and $\gamma_{xy}$ equally

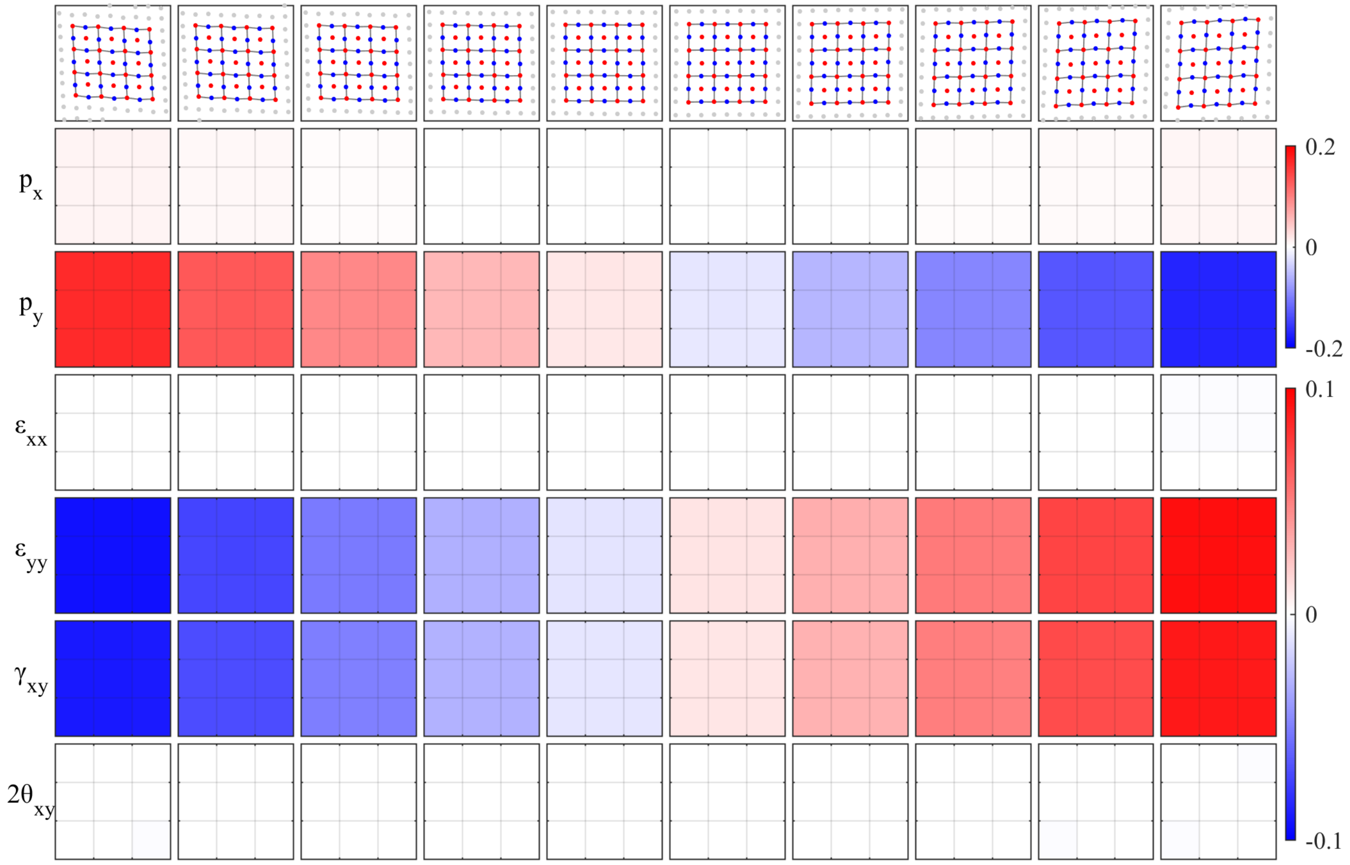


Figure S13: Changing $\varepsilon_{yy}$ and $\gamma_{xy}$ equally

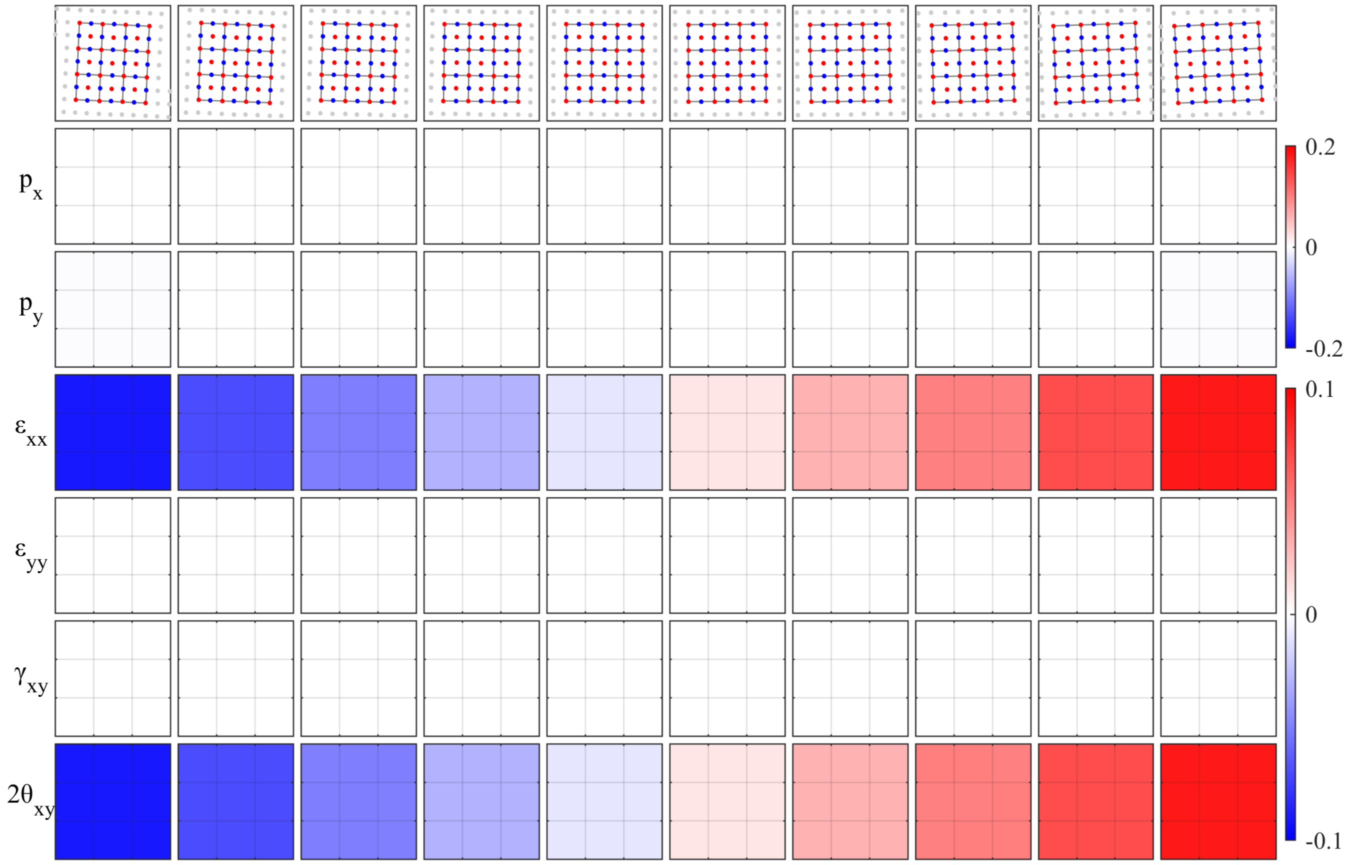


Figure S14: Changing $\varepsilon_{xx}$ and $2\theta_{xy}$ equally

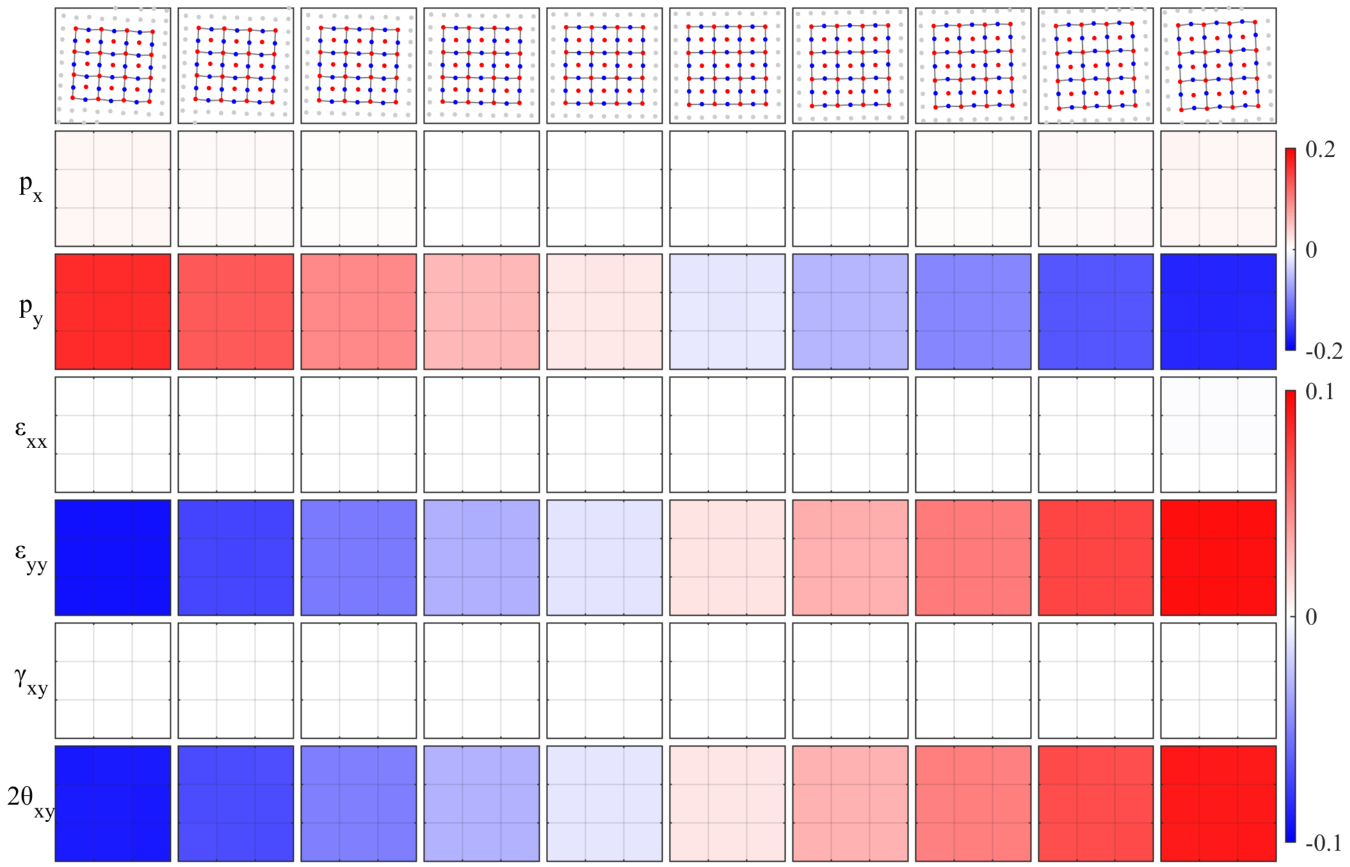


Figure S15: Changing $\varepsilon_{yy}$ and $2\theta_{xy}$ equally

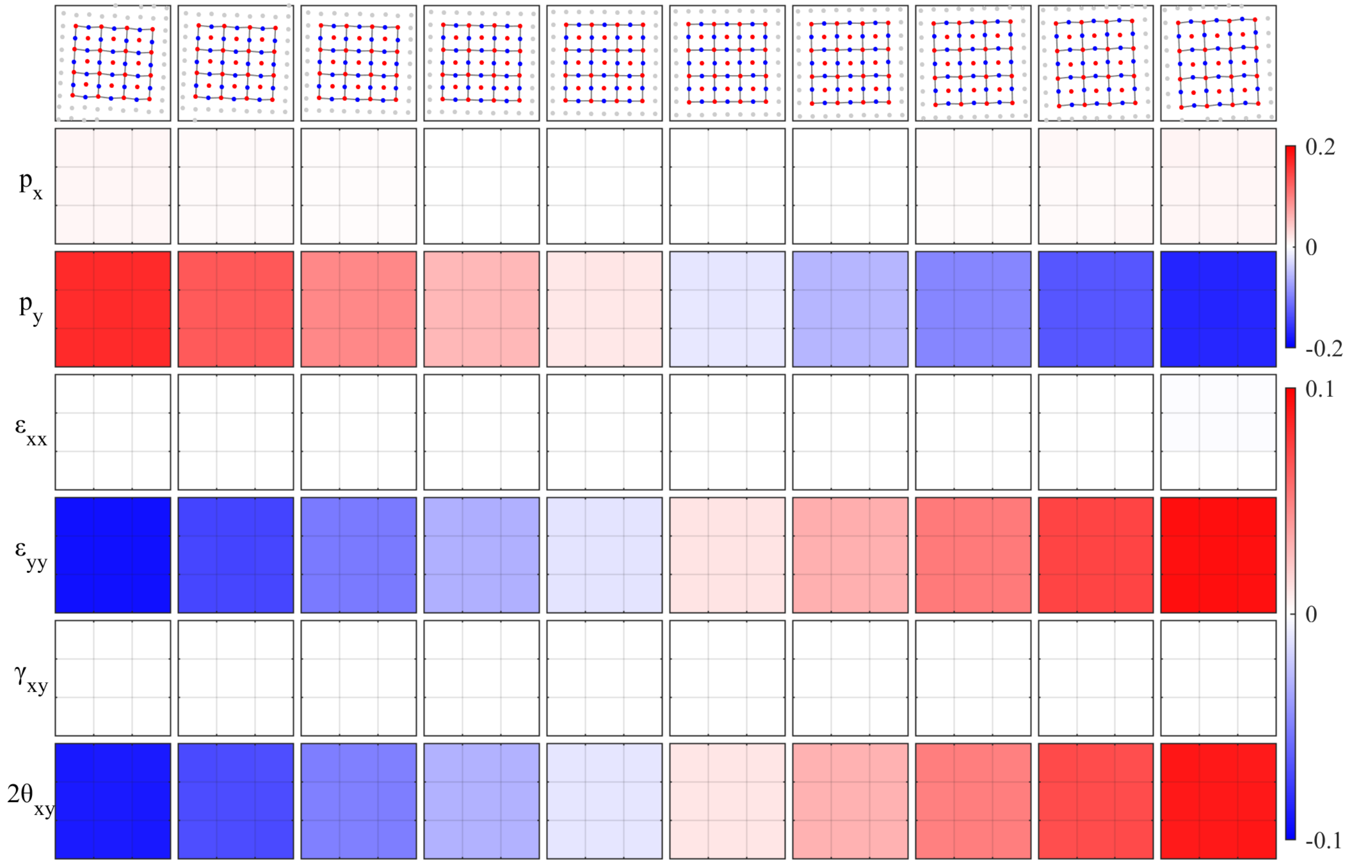


Figure S16: Changing $\gamma_{xy}$ and $2\theta_{xy}$ equally

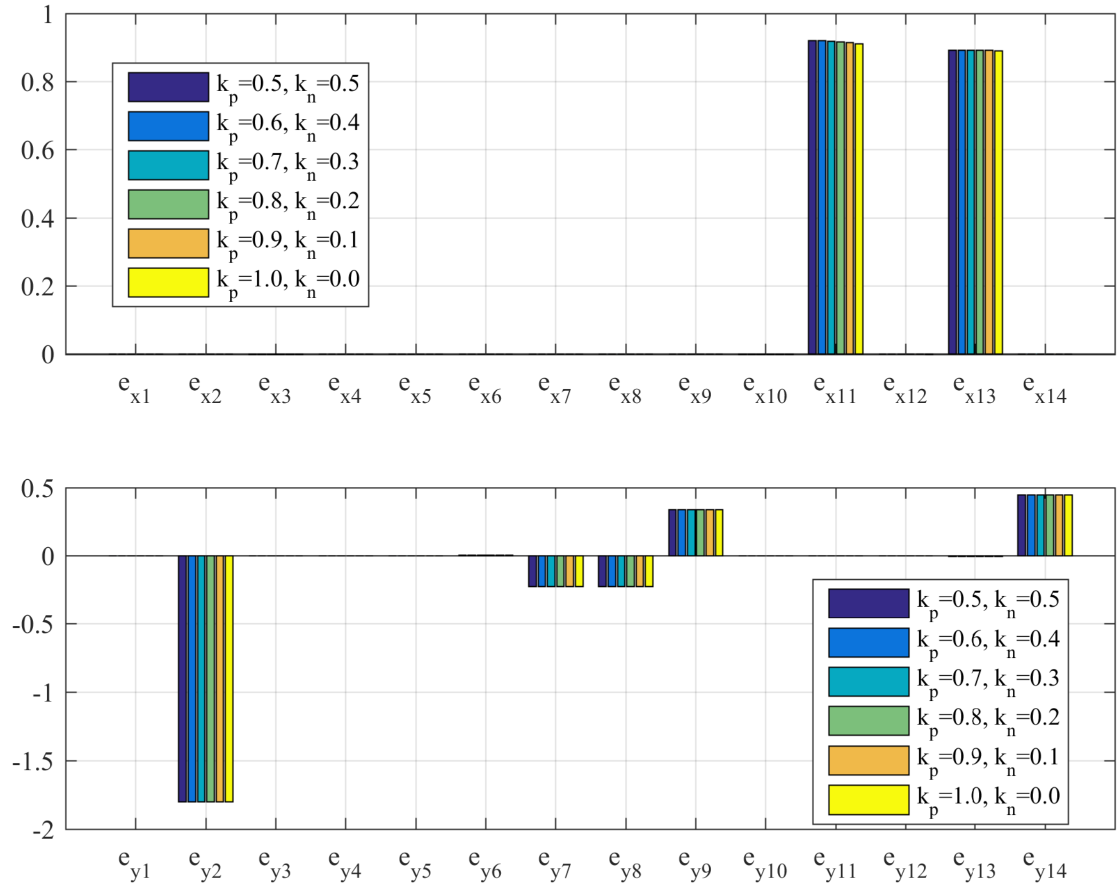


Figure S17: Piezoelectric coefficients for various diagonal spring combinations

# 5 Calculating process for the flexoelectric coefficients

The process of calculating the flexoelectric coefficients is similar to the process of the piezoelectric coefficients discussed in the previous section. For a given spring constant condition, its piezoelectric constants are calculated by the process described in the previous section. After that, a series of constant transverse strain gradient configurations are prepared from $-0.05/a$ to $0.05/a$ by $0.01/a$ step except the trivial zero strain gradient case. The Figure S18 shows the sample case of $k_{1x} = k_{2x} = k_{1y} = k_{2y} = 1$, $k_p = 0.9$, $k_n = 0.1$ that manifests the conventional linear flexoelectric effect only.

The data set of local dipole moments, local strain states, and local transverse strain gradient of $\frac{\Delta\varepsilon_{xx}}{\Delta y}$ which is defined in the Equation 24 are collected. The piezoelectric contribution to the local dipole moment is removed by an estimate based on the obtained piezoelectric coefficients and the local strain state. The remaining values are considered to be attributed to the flexoelectric effects. The Figure S19 shows the piezoelectric-effect-removed local dipole moments along the $y$-axis with respect to the local transverse strain gradient of $\frac{\Delta\varepsilon_{xx}}{\Delta y}$ for various spring constant conditions. Each relaxed configuration provides nine data points that are from each pole-free cell. The refined local $y$-dipole moment is fitted by the second order polynomial model with respect to the local transverse strain gradient, *i.e.*

$$p_{\text{u.c.}}^{\text{flexo}} = \mu^{(1)}\acute{\varepsilon} + \mu^{(2)}\acute{\varepsilon}^2, \tag{36}$$

where $\acute{\varepsilon} = \frac{\Delta\varepsilon_{xx}}{\Delta y}$ (equation 9 in the main letter). By this mean, the first order and the second order flexoelectric coefficients are obtained for the given spring constant condition. The flexoelectric coefficients are displayed in the Figure 6 in the main article.

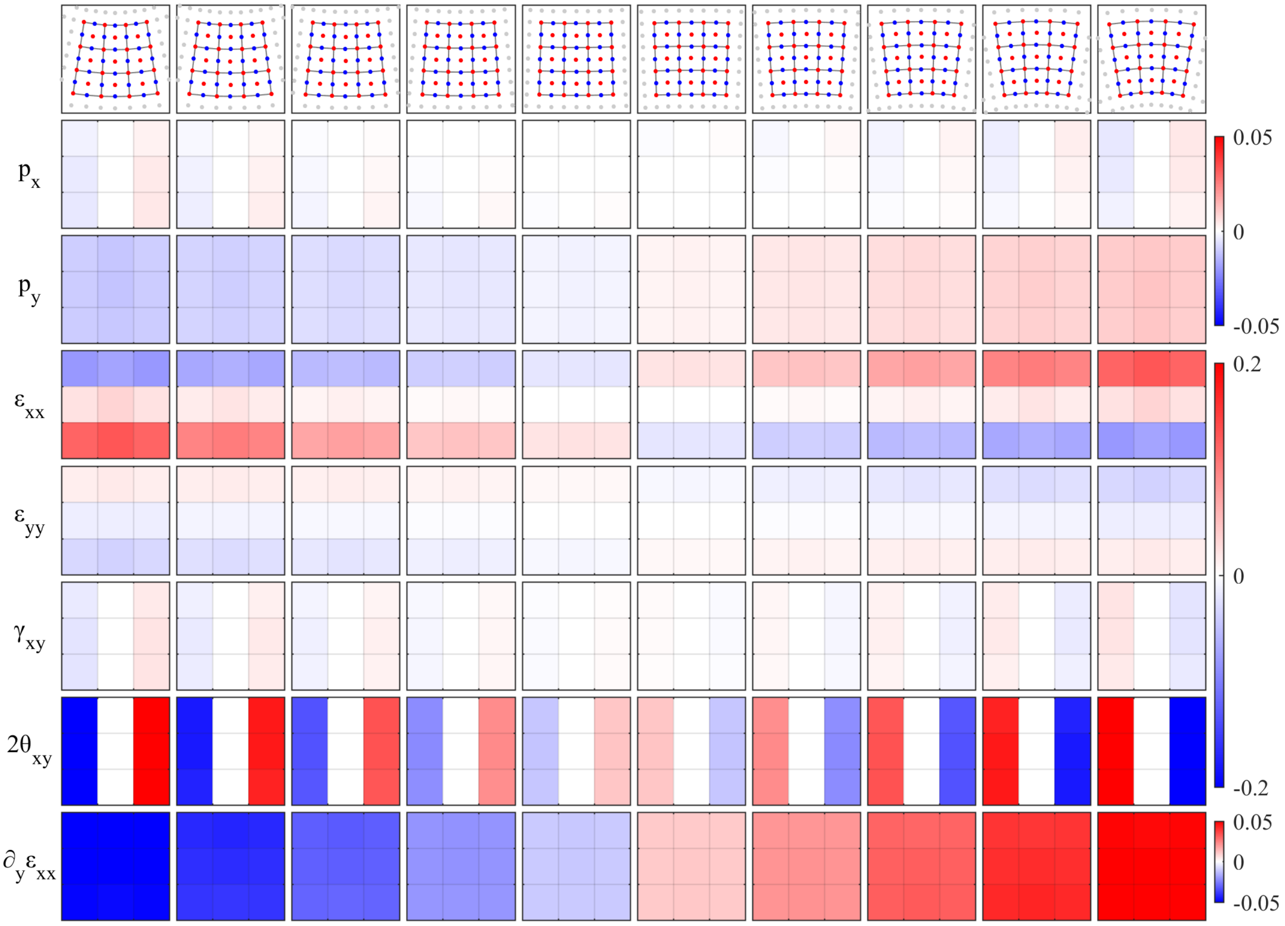


Figure S18: Series of relaxed configurations of various transverse strain gradient showing the linear flexoelectric effect. $(k_{1x} = k_{2x} = k_{1y} = k_{2y} = 1,\ k_p = 0.9,\ k_n = 0.1)$

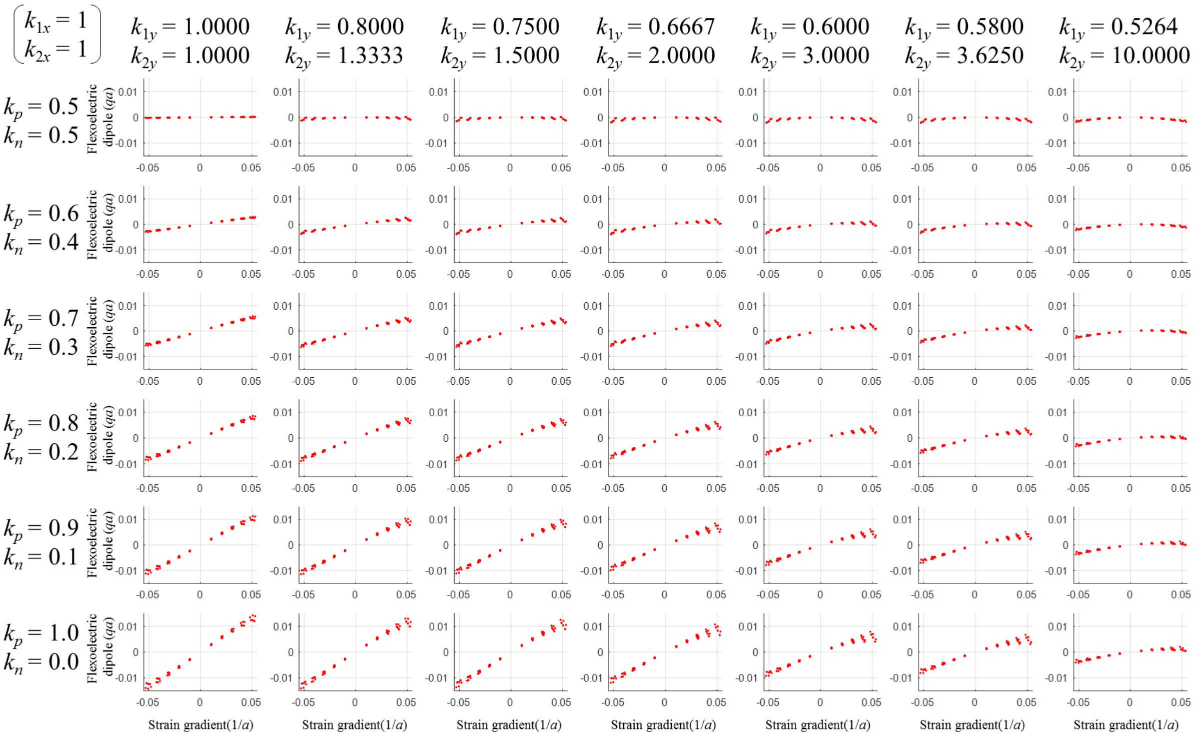


Figure S19: Local flexoelectric dipole moments with respect to local transverse strain gradient of $\frac{\Delta \varepsilon_{xx}}{\Delta y}$ for various spring constant configurations.

# 6 System size scaling

Unlike the polarization which is an intensive property, the induced dipole moment is an extensive property that scales to the size of a system. If the induced dipole moment does not scale to the size of the system, the quadratic flexoelectric effect term is not suitable to be included in the Landau free energy density function which is described by the intensive properties. In this section, we confirm that the induced quadratic flexoelectric dipole moment scales linearly to the system size. A series of systems, that are different in their size but same in applied strain gradients, are prepared. The spring constant condition is $k_{1x} = k_{2x} = 1$, $k_{1y} = 0.5264$, $k_{2y} = 10$ , $k_p = k_n = 0.5$. A single transverse strain gradient of $0.01/a$ is applied to the systems of various sizes containing 1-by-1, 2-by-2, 3-by-3, 5-by-5, 7-by-7, and 10-by-10 pole-free cells as shown in the Figure S20. Utilizing the piezoelectric coefficients (Table S1) and the local strain states, the local dipole moments induced by the piezoelectric effects are all removed cell by cell. After that, the total induced flexoelectric dipole moment can be analyzed with respect to the system size. In the Figures S21 and S22 show the map of the local dipole moment, local strain states, piezoelectric-effect-removed local dipole moments responsible for the flexoelectric effect, and the graph of total flexoelectric dipole moment with respect to the system size. Firstly, the $x$-flexoelectric dipole moment is zero as expected by the symmetry consideration. Since the inversion symmetry is broken along the $y$-axis only and the applied transverse strain gradient of $\frac{\Delta\varepsilon_{xx}}{\Delta y}$ does not distinguish positive and negative $x$-directions, the total $x$-dipole moment should be zero as shown in the graph in the bottom. Secondly, the magnitude of $y$-flexoelectric dipole moment increases linearly as the system size gets larger. The local flexoelectric moment maps show the spatially homogeneous feature, although the largest system size of 10-by-10 shows deviations from the linear trends for both cases. In addition, the local flexoelectric dipole moment map shows inhomogeneity at the boundary region. It is due to the nonlinear piezoelectric response under a huge strain that the second order polynomial description is insufficient. For the 10-by-10 pole-free cell system, the strain gradient of $0.01/a$ provides a huge strain ($\varepsilon_{xx}$) of $\pm 0.1$ near the top and bottom layers and a huge tilt ($2\theta_{xy}$) of $\pm 0.2$ near the left and right layers. Such large strain and tilt values exceed the fitting ranges that are used in the calculating process of piezoelectric coefficients. We expect that the higher order correction can overcome this deviation issue occurring in the large sized system.

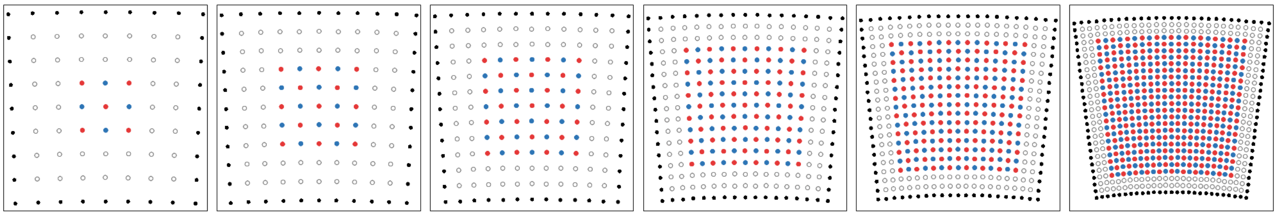

1-by-1 2-by-2 3-by-3 5-by-5 7-by-7 10-by-10

Figure S20: Relaxed configurations of various sizes under a constant strain gradient of $0.01/a$

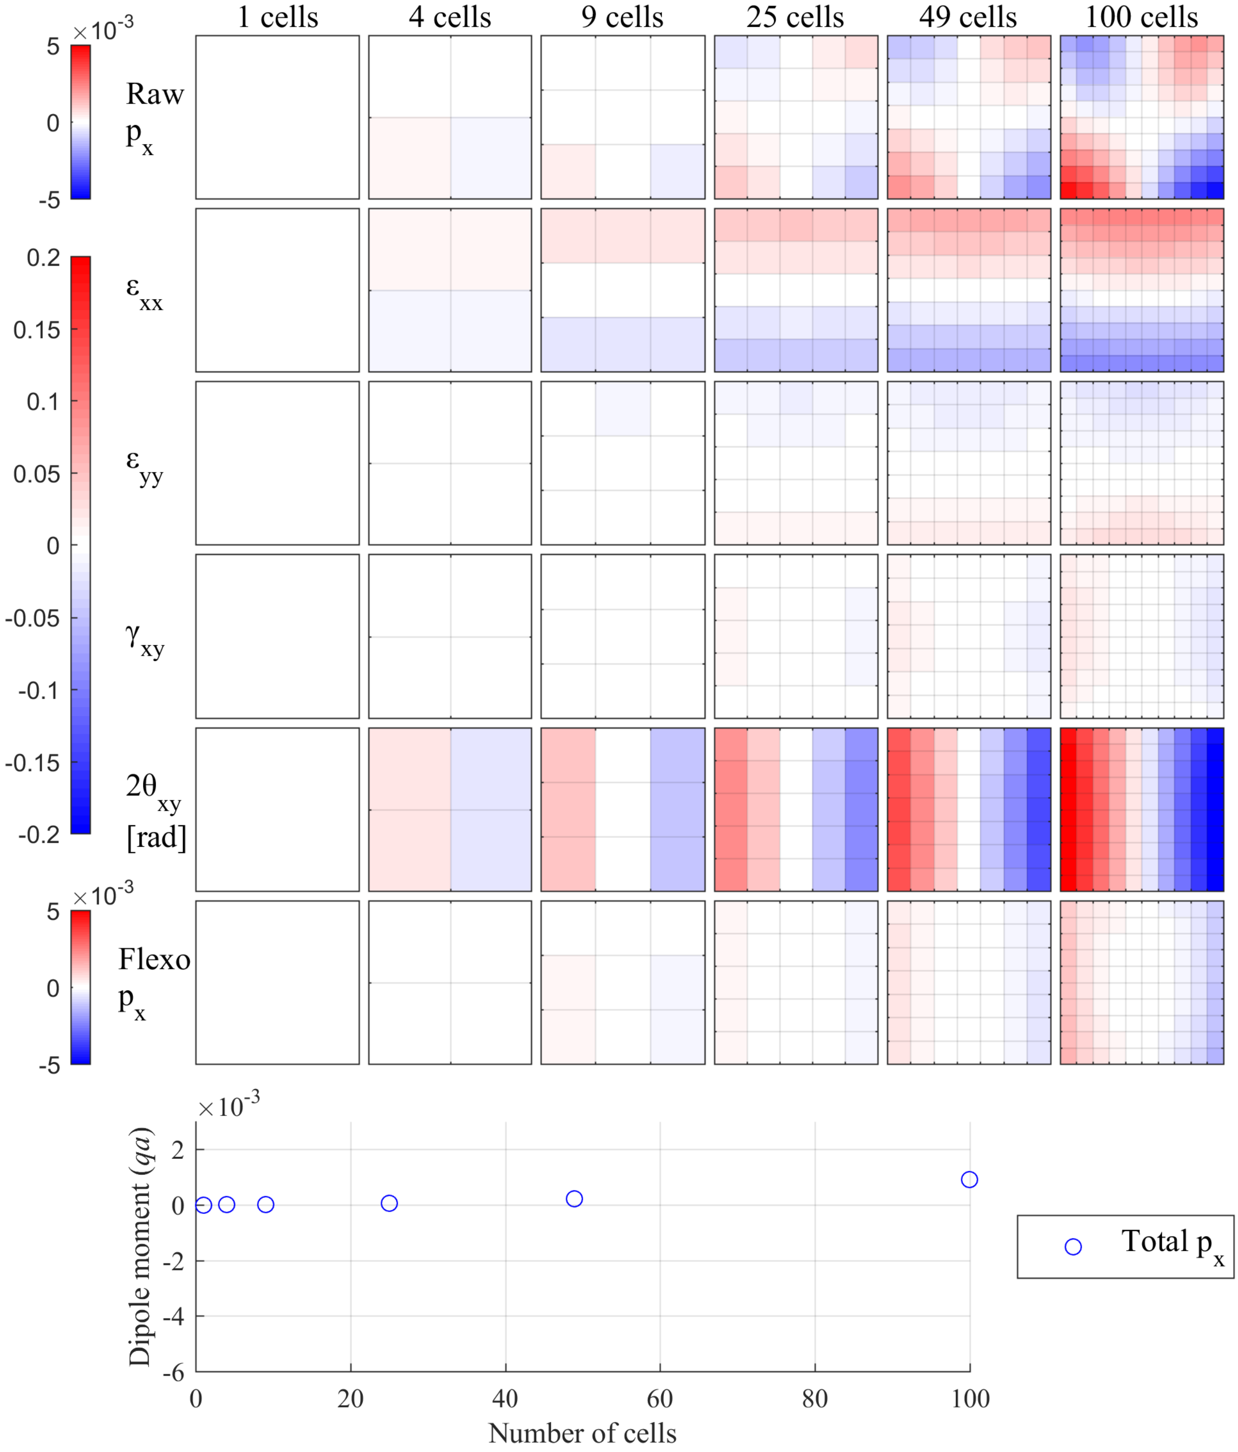


Figure S21: System size dependency of $x$-flexoelectric polarization

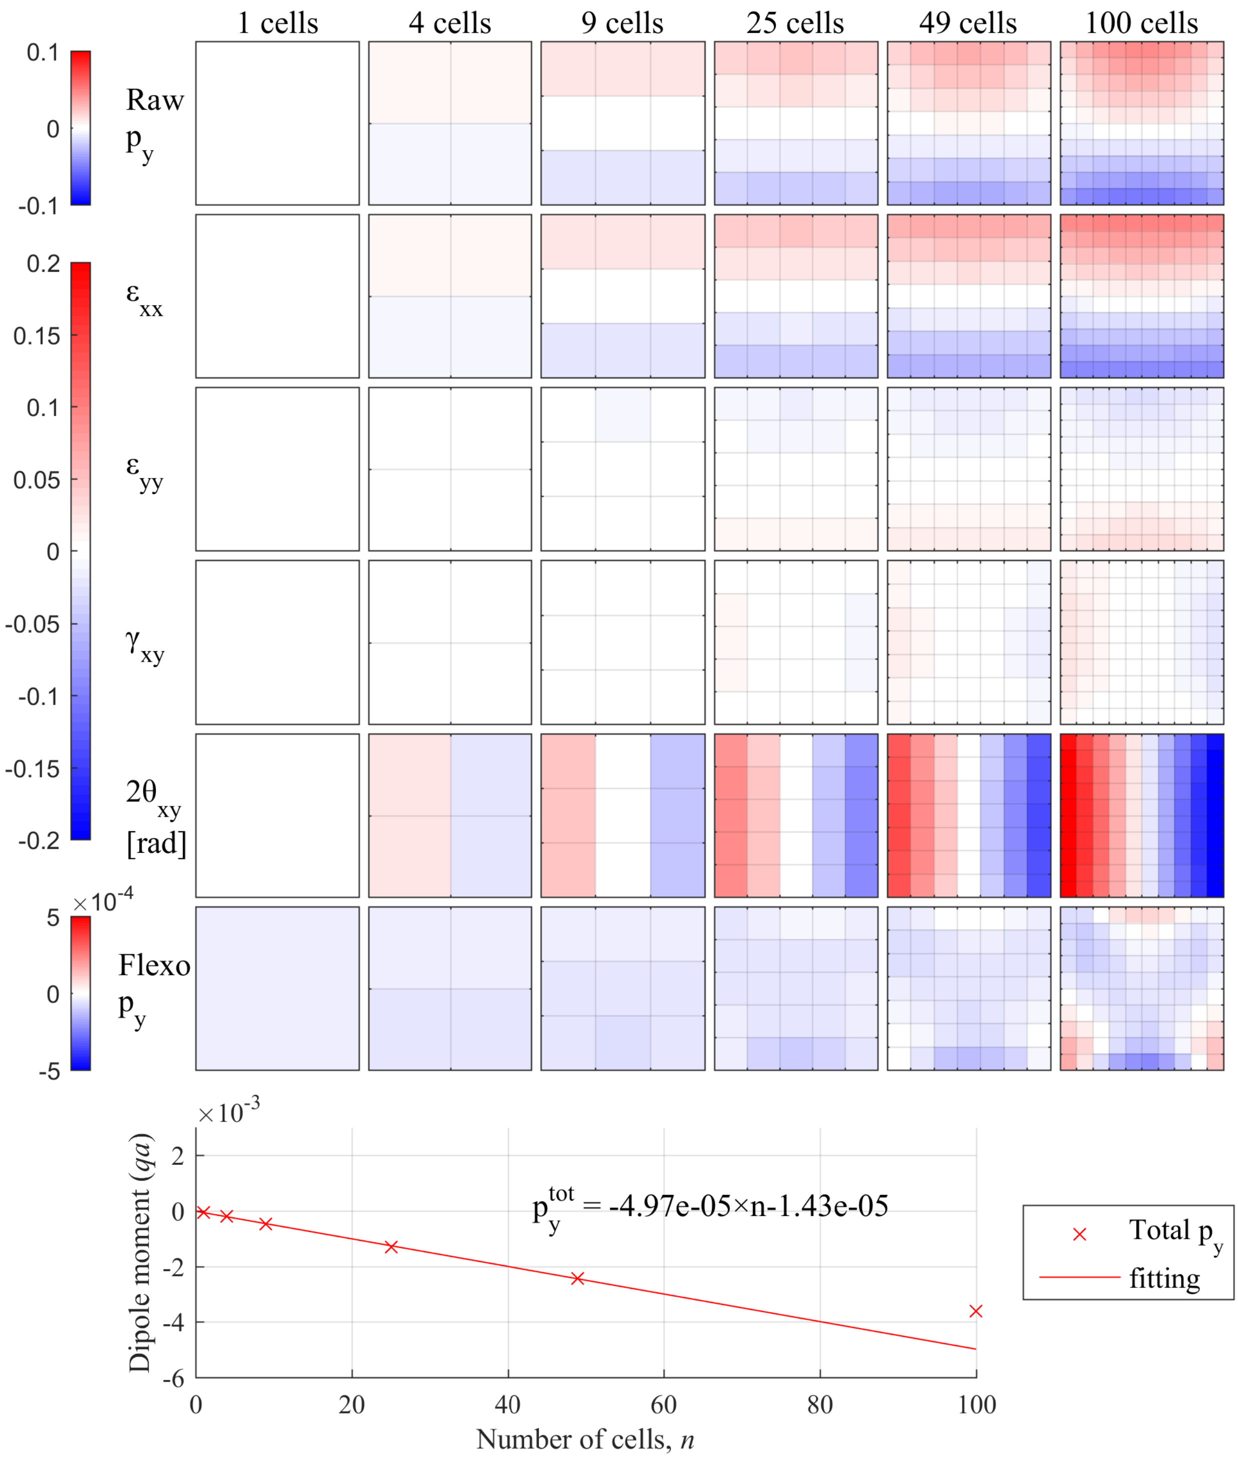


Figure S22: System size dependency of $y$-flexoelectric polarization
